# Supplementary material for: Two-Step SPLADE: Simple, Efficient and Effective Approximation of SPLADE
Source: arXiv:2404.13357 source file (2024-04-20)
Supplement: Supplementary file 1 [file appendix.tex]

%\newpage

\appendix

\section{Negative results with more complex static pruning alternatives}

To start, we would like to note something about our methods, \emph{they are simple}. Indeed, we focus on presenting a concise experimental setup of just 3 pruning techniques and their results for various retrieval methods. One main criticism is: why do we choose only these simple methods, while many others exist, with increasing complexity? In parallel, we actually tested a number of other techniques that did not work as well as the ones we just described, and require deeper investigation. In summary, we also tested: 
\begin{enumerate}
    \item Using \emph{different thresholds} for \emph{expansion and non-expansion terms} (in document-centric and agnostic pruning): Considering that expanded terms are less important compared to the non-expanded ones and thus could be more heavily pruned. We saw almost no difference to a single threshold.
    \item Term-centric pruning with \emph{varying quantiles} depending on the size of the term posting list: In (T) we prune all terms to a given quantile.  Another approach would be to vary the quantiles depending on the posting list length. No improvements were found compared to the simpler (T).
    \item Term-centric pruning to a maximum posting list size: Instead of choosing a quantile of the original posting list, one could use a desired maximum length. The results were worse than with a quantile-based approach.
    \item Reducing the scores during value agnostic pruning: When performing agnostic pruning we change the minimum score from 0 to the threshold score. Another solution would be to reduce all values so that the new threshold equals 0. This approach led to results worse than just keeping the minimum score as the threshold.
\end{enumerate}

\section{Experimental details}

Experiments are performed on a single machine, Intel(R) Xeon(R) Gold 6338 CPU @ 2.00GHz CPU, and evaluated using PISA. Full details for reproducing experiments are made available at the codebase: 
Inference time (i.e., the time to compute query term weights and expansion, if required) is disregarded for most of the experiments, as we only compare within the same retrieval model, thus having the same inference time. Inter-model comparison is only made with relative values. Latency is always reported as the average value across the set of queries in each experiment and measured in milliseconds. Retrieval is performed with MaxScore dynamic pruning.

\begin{figure*}[ht]
     \centering
     \begin{subfigure}[t]{\textwidth}
         \centering
\adjustbox{max width=\textwidth}{%
%         \raisebox{120px}{%
         \input{tikz/with_reranking/MSMARCO/legend.tex}}
%}
     \end{subfigure}
     \begin{subfigure}[t]{0.3\textwidth}

         \centering
\adjustbox{max width=\textwidth}{%
         \input{tikz/with_reranking/MSMARCO/pisa2.tex}
         }
     \end{subfigure}
      \caption{Two stage SPLADE over MSMARCO. Without log on the xaxis}
     \label{fig:with_rerank_msmarco_wout}
\end{figure*}

\section{Index size}

In the main paper, we consider solely the retrieval inference time but ignored the index size reduction that is incurred due to pruning. We present the values in Figure~\ref{fig:relative_effectiveness} which is similar to Figure 1 of the main paper, but using relative index size instead of relative latency. We note that the compression effect is less pronounced than the speedup for most retrieval and pruning method combinations, especially for BM25 which is already pretty well compressed. The only exceptions are using SPLADE for retrieval, which we posit is because of the large size of the original index and the use of term-based pruning which makes sense as smaller posting lists are easier to compress.

\section{Full TREC-DL results}

In this Section, we present extensions to Table 1 of the full paper, where we consider all retrievers and all pruning methods. Results are presented in tables~\ref{tab:trec_bm25_full},~\ref{tab:trec_unicoil_full},~\ref{tab:trec_deepimpact_full}, and ~\ref{tab:trec_splade_full}. Overall we see the same results as in the shortened table of the full paper and the MSMARCO figure: we are able to get 2x speedup with $\leq 2\%$ loss of effectiveness and 4x speedup with $\leq 8\%$ loss of effectiveness with pretty much all pruning methods over all learned sparse retrieval models, however, we see that some conclusions could change, as for example, TREC-DL and SPLADE term-based pruning can sometimes be more effective than the other methods and that sometimes evaluation on TREC-DL may be skewed by a few queries, leading to a few results outside of the expected: ``more pruning equals faster and more approximate method''. 

\input{appendix_tables/TREC/bm25}

\input{appendix_tables/TREC/unicoil}

\input{appendix_tables/TREC/deepimpact}

\input{appendix_tables/TREC/splade}
